# Supplementary material for: An End-to-End AI-Based Framework for Automated Discovery of CEST/MT MR Fingerprinting Acquisition Protocols and Quantitative Deep Reconstruction (AutoCEST)
Source: arXiv:2107.04737 ancillary file (2021-07-10)
Supplement: Supplementary file 1 [file Supporting_Information.pdf]

**Supporting Information Table S1. Detailed properties of the simulated data used for training AutoCEST.**

| Compound of interest | Iohexol | pCr | L-arginine | BSA - amide | BSA - amine | BSA - rNOE | In Vivo MT | In Vivo Amide*** |
|---|---|---|---|---|---|---|---|---|
| Water $T_1$ (ms) | 2100:50:2700* | 3300:50:3800 | 2500:50:3300 | 2000:50:3400 | 2600:50:3400 | 2600:50:3400 | 1300:100:2600 | 1300:200:2500 |
| Water $T_2$ (ms) | 200:25:650 | 1000:50:1600 | 600:50:1200 | 50:10:300 | 50:10:300 | 50:10:300 | 40:10:130 | 40:20:120 |
| Solute/semi-solid $T_1$ (ms) | 2200 | 1000 | 2800 | Equal to water $T_1$[64] | Equal to water $T_1$[64] | Equal to water $T_1$[64] | Equal to water $T_1$[64] | Equal to water $T_1$[64] |
| Solute/semi-solid $T_2$ (ms) | 40 | 500[40] | 40 | 1 | 1 | 0.5[65] | 0.04** | 1 |
| Solute/semi-solid chemical shift (ppm) | 4.3 | 2.6 | 3 | 3.5 | 2.75 | -3.5 | -2.5 | 3.5 |
| Number of exchangeable protons | 2 | 1 | 3 | 1 | 1 | 1 | 1 | 1 |
| $k_{sw}$ / $k_{ssw}$ (Hz) | 10:10:300 | 50:5:200 | 100:10:1400 | 5:5:100 | 50:50:1500 | 5:5:100 | 5:5:100 | 5:5:100 |
| Solute/semi-solid concentration (mM) | 10:5:100 | 2:2:150 | 10:5:120 | 100:50:1000 | 20:20:600 | 50:50:1000 | 2k:2k:30k | 100:50:1000 |
| Optimized parameters and constratints (if any) | $B_1 \leq 6$ μT | $B_1 \leq 1.5$ μT<br>$T_{sat} \leq 5$s<br>$T_{rec} \leq 5$s | $B_1 \leq 6$ μT<br>$1.5s \leq T_{sat} \leq 3s$<br>$1.5s \leq T_{rec} \leq 2.5s$<br>FA<br>$\omega_{rf}$ | $B_1 \leq 4$ μT | $B_1 \leq 6$ μT | $B_1 \leq 4$ μT | $B_1 \leq 4$ μT<br>10 ppm $\leq \omega_{rf} \leq$ 75 ppm | $B_1 \leq 2$ μT |
| Fixed acquisition parameters | $T_{sat}$ = 2.5s<br>$T_{rec}$ = 1s<br>$\omega_{rf}$ = 4.3 ppm<br>FA = 90° | $\omega_{rf}$ = 2.6 ppm<br>FA = 90° | none | $T_{sat}$ = 2.5s<br>$T_{rec}$ = 1s<br>$\omega_{rf}$ = 3.5 ppm<br>FA = 90° | $T_{sat}$ = 2.5s<br>$T_{rec}$ = 1s<br>$\omega_{rf}$ = 2.75 ppm<br>FA = 90° | $T_{sat}$ = 2.5s<br>$T_{rec}$ = 1s<br>$\omega_{rf}$ = -3.5 ppm<br>FA = 90° | $T_{sat}$ = 2.5s<br>$T_{rec}$ = 1s<br>FA = 90° | $T_{sat}$ = 2.5s<br>$T_{rec}$ = 1s<br>$\omega_{rf}$ = 3.5 ppm<br>FA = 90° |
| Total number of simulated signals | 140,790 | 332,475 | 665,873 | 286,520 | 397,800 | 176,800 | 42,000 | 532,000 |
| Time required for AutoCEST to generate the optimized acquisition schedule (using a Linux Laptop with 8 CPUs) | 32 min | 2.50 hrs | 5.58 hrs | 2.38 hrs | 3.28 hrs | 1.61 hrs | 22 min | 4.07 hrs |

*The notation x:y:z represents a discrete range of values between [x, z] with y increments.
** The Bloch-McConnell equations based data generator yielded a Lorentzian line-shape for the semi-solid pool. To generate a linewidth equivalent to the commonly reported super-Lorentzian of 10 μs[52], a four times higher value (40 μs) was input to the dictionary generator[64].
*** A 3-pool scenario was simulated, by including both the amide and MT pool parameters, as described in the in-vivo MT column.

**Supporting Information Table S2**. **Comparison of the concentrations and proton chemical exchange rates determined by AutoCEST, CEST-MRF, and QUESP.**

| Phantom | Ground truth | | QUESP - ground truth concentration as input | QUESP - simultaneous estimation of concentration and exchange rate | | AutoCEST | | Unoptimized CEST-MRF | |
|---|---|---|---|---|---|---|---|---|---|
| | **Concentration (mM)** | **pH** | **$k_{sw}$ (Hz)** | **Concentration (mM)** | **$k_{sw}$ (Hz)** | **Concentration (mM)** | **$k_{sw}$ (Hz)** | **Concentration (mM)** | **$k_{sw}$ (Hz)** |
| pCr | 50 | 7.2 | 264±158 | 27±26 | 257±156 | 55±13 | 274±21 | 149±9 | 199±11 |
| | 25 | 7.2 | 267±356 | 13±28 | 267±356 | 27±7 | 252±13 | 147±8 | 179±15 |
| | 12.5 | 7.2 | 238±650 | 8±45 | 193±610 | 14±9 | 223±22 | 149±4 | 154±16 |
| Iohexol | 20 | 7.0 | 196±24 | 10±5 | 271±108 | 20±25 | 207±44 | 97±10 | 134±30 |
| | 80 | 7.0 | 178±12 | 47±5 | 232±21 | 81±21 | 223±40 | 98±8 | 228±25 |
| | 40 | 7.0 | 179±14 | 21±3 | 241±32 | 36±9 | 231±17 | 94±13 | 172±27 |
| | 20 | 7.4 | 300±287 | 27±44 | 300±503 | 19±10 | 295±20 | 100±0 | 300±0 |
| | 20 | 5.9 | 23±2734 | 15±1271 | 29±2305 | 23±9 | 76±30 | 100±4 | 72±19 |
| | 20 | 6.8 | 223±24 | 10±4 | 294±87 | 22±8 | 215±17 | 99±6 | 148±25 |
| L-arg | 50 | 5.0 | 341±43 | 41±5 | 340±43 | 53±7 | 294±25 | 106 ± 15 | 303 ± 35 |
| | 100 | 5.0 | 357±28 | 93±10 | 349±49 | 101±7 | 335±14 | 112 ± 15 | 403 ± 33 |
| | 25 | 5.1 | 343±46 | 18±2 | 343±46 | 26± 4 | 238 ± 22 | 106 ± 15 | 227 ± 22 |
| | 50 | 5.0 | 363±42 | 43±4 | 365±42 | 51 ± 5 | 318 ± 28 | 104 ± 18 | 326 ± 38 |
| | 50 | 4.0 | 176±41 | 36±10 | 176±41 | 51 ± 7 | 153 ± 22 | 118 ± 8 | 154 ± 19 |
| | 50 | 4.5 | 231±39 | 36±7 | 232±39 | 53 ± 8 | 196 ± 32 | 117 ± 7 | 200 ± 20 |
| | 50 | 5.4 | 621±122 | 51±4 | 549±65 | 61 ± 4 | 518 ± 23 | 79 ± 15 | 605 ± 50 |
| | 50 | 5.0 | 363±20 | 37±4 | 378±44 | 50 ± 4 | 334 ± 23 | 98 ± 20 | 351 ± 46 |
| | 50 | 6.0 | 870±135 | 47±2 | 882±117 | 53 ± 4 | 892 ± 45 | 63 ± 5 | 1119 ± 66 |
| **Absolute error** | | | | 11.03 ± 7.77 (mM) | 23.94 ± 29.54 (Hz) | 2.42 ± 2.53 (mM) | 35.8 ± 29.3 (Hz) | 65.19 ± 34.48 (mM) | 58.2 ± 56.76 (Hz) |
| **Correlation with known concentrations or QUESP** | | | | r=0.918 p<0.0001 CI=[0.790, 0.969] | r=0.980 p<0.0001 CI=[0.947, 0.993] | r=0.992 p<0.0001 CI=[0.977, 0.997] | r=0.971 p<0.0001 CI=[0.923, 0.989] | r=-0.161 p=0.522 CI=[-0.58, 0.33] | r=0.959 p<0.0001 CI=[0.891, 0.985] |

CI = confidence interval

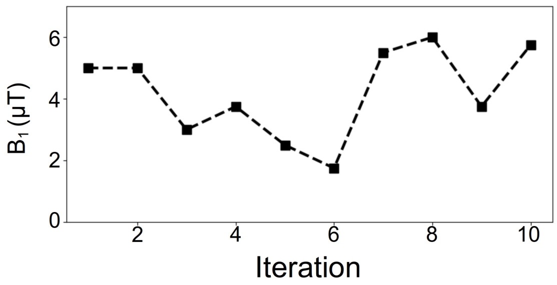


**Supporting Information Figure S1.** A previously reported phantom acquisition schedule[22], shortened to N=10 images and used as a reference unoptimized CEST-MRF protocol. The saturation pulse duration was 3s, the recovery time was 1s, the readout flip angle was 60°, and the saturation pulse frequency was set to the chemical shift of each imaged phantom.
